# Supplementary material for: Hi-WM: Human-in-the-World-Model for Scalable Robot Post-Training
Source: arXiv:2604.21741 source file (2026-05-05)
Supplement: Supplementary file 1 [file appendix.tex]

\appendix

\section{Limitation}
